# Supplementary material for: FiGURe: Simple and Efficient Unsupervised Node Representations with Filter Augmentations
Source: arXiv:2310.01892 source file (2023-10-04)
Supplement: Supplementary file 1 [file appendix.tex]

\begin{table}[!ht]
    
    \centering
    \caption{Mean epoch time (in milliseconds) averaged across 20 trials with different hyperparameters. Importantly, even though our method is slower at 512 dimensions, using 32 and 128 dimensional embeddings significantly reduces the training time, with mininal drop in performance as demonstrated in Table \ref{tab:rff_table_32} and Table \ref{tab:rff_table_128}}   \resizebox{\linewidth}{!}{   
    \begin{tabular}{lllllll}
    \hline
         & Dim Size & \dgi & \mvgrl & \grace & \sugrl & \ourmethod \\ \hline
        \cora & 512 & 38.53(0.77) & 75.29(0.56) & 51.20(6.84) & 15.92(4.11) & 114.38(0.51) \\ 
        ~ & 128 & 6.82(0.51) & 12.41(0.66) & 20.79(2.24) & 9.46(3.77) & 20.10(0.46) \\ 
        ~ & 32 & 4.10(0.52) & 6.13(0.23) & 14.96(2.11) & 9.45(3.96) & 11.54(0.34) \\ \hline
        \citeseer & 512 & 52.98(1.15) & 102.41(0.99) & 77.16(7.20) & 24.38(4.93) & 156.24(0.56) \\ 
        ~ & 128 & 10.38(0.89) & 18.28(0.86) & 29.20(2.19) & 14.80(5.49) & 30.30(0.60) \\ 
        ~ & 32 & 5.87(0.79) & 9.08(0.25) & 18.16(2.09) & 9.43(3.68) & 17.16(0.51) \\ \hline
        \squirrel & 512 & 87.06(2.07) & 168.24(2.08) & 355.27(67.34) & 33.64(6.94) & 257.65(0.76) \\ 
        ~ & 128 & 16.58(1.90) & 28.27(1.90) & 104.86(17.52) & 15.62(3.66) & 47.72(1.40) \\ 
        ~ & 32 & 8.11(0.45) & 12.36(0.51) & 41.05(5.13) & 11.47(4.11) & 23.52(1.14) \\ \hline
        \chameleon & 512 & 33.08(0.49) & 64.71(1.05) & 85.05(14.11) & 16.91(5.91) & 98.36(0.64) \\ 
        ~ & 128 & 6.34(0.48) & 11.51(0.77) & 27.56(3.98) & 11.26(5.13) & 18.56(0.39) \\ 
        ~ & 32 & 4.13(0.37) & 6.51(0.24) & 15.89(2.21) & 9.17(3.84) & 11.63(0.48) \\ \hline
    \end{tabular}}
\label{tab:computational_efficiency}
\end{table}

\begin{table}[!ht]
    
    \small
    \centering
    \caption{Node classification accuracy results with and without using Random Fourier Feature projections (on 128 dimensions). A higher number means better performance. Here as well, the performance is improved by using RFF in almost all cases reinforcing the need for this transformation}
    \begin{tabular}{llllll}
    \hline
         & RFF & \cora & \citeseer  & \squirrel & \chameleon \\ \hline
        \dgi & No & \tblfirst{84.99 (1.36)} & 72.22 (2.50) & 34.22 (1.47) & 49.82 (2.96) \\ 
        ~ & Yes & 84.16 (2.11) & \tblfirst{72.65 (1.52)} & \tblfirst{37.97 (1.41)} & \tblfirst{57.72 (2.03)} \\ \hline
        \mvgrl & No & \tblfirst{84.99 (1.34)} & \tblfirst{73.16 (1.21)} & 33.81 (1.85) & 52.00 (2.87) \\ 
        ~ & Yes & 84.00 (1.43) & 72.46 (1.62) & \tblfirst{38.77 (0.97)} & \tblfirst{58.46 (2.81)} \\ \hline
        \sugrl & No & \tblfirst{71.49 (1.15)} & \tblfirst{63.85 (2.27)} & 38.04 (1.17) & 53.03 (1.73) \\ 
        ~ & Yes & 71.41 (1.40) & 63.06 (2.22) & \tblfirst{43.24 (1.63)} & \tblfirst{57.04 (1.78)} \\ \hline
        \grace & No & \tblfirst{80.87} (1.49) & 62.52 (3.57) & 41.25 (1.32) & 63.14 (1.89) \\ 
        ~ & Yes & 79.70 (1.91) & \tblfirst{64.47 (2.12)} & \tblfirst{52.29 (1.81)} & \tblfirst{68.90 (2.05)} \\ \hline
        \ourmethod & No & 84.73 (1.13) & 73.07 (1.13) & 41.06 (1.51) & 59.08 (3.36) \\ 
        ~ & Yes & \tblfirst{86.14 (1.13)} & \tblfirst{73.34 (1.91)} & \tblfirst{48.78 (2.48)} & \tblfirst{66.03 (2.19)} \\ \hline
    \end{tabular}
\label{tab:rff_table_128}
\end{table}

% As anticipated, the computation time exhibited a substantial decrease as the embedding dimension decreased from 512 to 128, and further to 32. This observation aligns with our expectations and highlights the advantages of working with lower dimensional embeddings. The reduced computation time associated with lower dimensional embeddings underscores their usefulness in practical applications, especially when efficiency is a priority. Moreover, this finding serves as a motivation for incorporating RFF projections in the learning process. By leveraging RFF, it becomes possible to recover and enhance performance while operating with lower dimensional embeddings. 

\subsection{RQ6: Which is better, RFF projection followed by combination vs combination followed by RFF?} 
\label{subsec:exp_pre_vs_post}
\begin{table}[!ht]
    
    \small
    \centering
    \caption{Pre RFF vs Post RFF on 32 dimensions}
    \begin{tabular}{llllll}
    \hline
        & \cora & \citeseer & \squirrel & \chameleon \\ \hline
        Pre & 82.56 (0.87) & 71.25 (2.20) & 48.89 (1.55) & 65.66 (2.52) \\ 
        Post & 81.79 (2.12) & 71.90 (1.97) & 45.33 (1.60) & 0 (0) \\ \hline
    \end{tabular}
    \label{tab:pre_vs_post_32}    
\end{table}

There are two methods of combining the lower dimensional representations obtained from different filters. In the first method, the learnt embeddings are first individually transformed to the higher dimensional RFF space, and then the combination weights and and logistic regression weights are learned together. The second method involves first combining the embeddings using a sum, followed by a projection into the RFF space, and then the logistic regression layer. In our previous results we have used the first method. To answer the question, whether the second method can be used as well, we conducted an experiment, the results of which are in Table \ref{tab:pre_vs_post_32}. Both methods appear to give similar results, and

%%%%%%%%%%%%%%%%%%%%%%%%%%%%%

\begin{table}[!ht]
    
    \centering
    \caption{Node classification accuracy results on Heterophilic Datasets. @32 and @128 represent 32 and 128 dimensional representations respectively. All others are at 512 dimensions. A higher number means better performance. \ourmethod~either outpereforms or is competive with the baselines.}
    \resizebox{\linewidth}{!}{
    \begin{tabular}{llllllll}
    \hline
         & \squirrel & \chameleon & \romanempire & \minesweeper & \texas & \wisconsin & \cornell \\ \hline
        \gcn            & 47.78 (2.13) & 62.83 (1.52) & 73.69 (0.74) & 89.75 (0.52) & 59.73 (4.89) & 58.82 (4.89) & 60.00 (4.90) \\          
        \deepwalk       & 38.66 (1.44) & 53.42 (1.73) & 13.08 (0.59) & 79.96 (0.08) & 55.41 (3.68) & 50.78 (5.44) & 57.57 (3.43) \\ 
    \nodevec            & 42.60 (1.15) & 54.23 (2.30) & 12.12 (0.30) & 80.00 (0.00) & 30.00 (5.60) & 20.00 (4.19) & 29.73 (7.83) \\ 
        \dgi            & 39.61 (1.81) & 59.28 (1.23) & 47.54 (0.76) & 82.51 (0.47) & 58.38 (7.76) & 51.96 (5.42) & 54.32 (6.89) \\ 
        \mvgrl          & 39.90 (1.39) & 54.61 (2.29) & 68.50 (0.38) & 85.60 (0.35) & 60.54 (5.69) & 60.98(6.04) & 63.24 (2.48) \\ 
        \grace          & \tblfirst{53.15 (1.10)} & 68.25 (1.77) & 47.83 (0.53) & 80.22 (0.45) & 64.05 (6.17) & 61.37 (2.78) & 55.68 (5.01) \\ 
        \sugrl          & 43.13 (1.36) & 58.60 (2.04) & 39.40 (0.49) & 82.40 (0.58) & 57.84 (6.96) & 54.12 (6.02) & 53.51 (5.51) \\ 
        \ourmethod @32  & \tblthird{48.89 (1.55)} & 65.66 (2.52) & 67.67 (0.77) & 85.28 (0.71) & 0 & 0 & 0 \\
        \ourmethod @128 & 48.78 (2.48) & 66.03 (2.19) & 68.10 (1.09) & 85.16 (0.58) & 0 & 0 & 0 \\  
        \ourmethod      & \tblsecond{52.23 (1.19)} & 68.55 (1.87) & 70.99(0.52) & 85.58 (0.49) & 83.78 (5.92) & 79.80 (5.62) & 77.30 (6.30) \\ \hline
    \end{tabular}}
    \label{tab:main_table_heterophilic}
\end{table}

\begin{table}[!ht]
    
    \small
    \centering
    \caption{Node classification accuracy results on Heterophilic Datasets. @32 and @128 represent 32 and 128 dimensional representations respectively. All others are at 512 dimensions. A higher number means better performance. \ourmethod~either outpereforms or is competive with the baselines.}
    \begin{tabular}{llllllll}
    \hline
         & \cora  & \citeseer & \pubmed & \computers \\ \hline
        \gcn & 87.36 (0.91) & 76.47 (1.34) & 88.41 (0.46) & 82.50 (1.23) \\ 
        \deepwalk & 83.64 (1.85) & 63.66 (3.36) & 80.85 (0.44) & 76.46 (1.11) \\ 
        \nodevec & 78.19 (1.14) & 57.45 (6.44) & 73.24 (0.59) & 72.16 (2.14) \\ 
        \dgi & 84.57 (1.22) & 73.96 (1.61) & 86.57 (0.52) & 79.87 (2.46) \\ 
        \mvgrl & 86.22(1.30) & 75.02 (1.72) & 87.12 (0.35) & 81.19(1.98) \\ 
        \grace & 84.79  (1.51) & 67.60 (2.01) & 87.04 (0.43) & 77.96  (1.97) \\ 
        \sugrl & 81.21 (2.07) & 67.50 (1.62) & 86.90 (0.54) & 68.22  (1.36) \\ 
        \ourmethod @32 & 82.56 (0.87) & 71.25 (2.20) & 84.18 (0.53) & 0  \\
        \ourmethod @128 & 86.14 (1.13) & 73.34 (1.91) & 85.41 (0.52) & 0 \\  
        \ourmethod & 87.00 (1.24) & 74.77 (2.00) & 88.60 (0.44) & 82.05 (1.25) \\ \hline
    \end{tabular}
    \label{tab:main_table_homophilic}
\end{table}

%%%%%%%%%%$

\begin{table}[!ht]
    
    \centering
    \caption{Node Classification accuracy percentage delta with \ourmethod~across different datasets and methods. Each cell represents the gain in performance that \ourmethod has over method in the column header on the dataset in the row header. The performance deltas are averaged across each dataset for every method and reported in the last row.}
    \resizebox{\linewidth}{!}{
    \begin{tabular}{cccccccc}
    \hline
        . & DeepWalk & Node2Vec & DGI & MVGRL & GRACE & SUGRL & GCN \\ \hline
        Squirrel & 13.57 & 9.63 & 12.62 & 12.33 & -0.92 & 9.1 & 4.45 \\ 
        Chameleon & 15.13 & 14.32 & 9.27 & 13.94 & 0.3 & 9.95 & 7.12 \\ 
        Roman-empire & 57.91 & 58.87 & 23.45 & 2.49 & 23.16 & 31.59 & -2.7 \\ 
        Minesweeper & 5.62 & 5.58 & 3.07 & -0.02 & 5.36 & 3.18 & -4.17 \\ 
        Cora  & 3.36 & 8.81 & 2.43 & 0.78 & 2.21 & 5.79 & -0.36 \\ 
        Citeseer & 11.11 & 17.32 & 0.81 & -0.25 & 7.17 & 7.27 & -1.7 \\ 
        Pubmed & 7.75 & 15.36 & 2.03 & 1.48 & 1.56 & 1.7 & 0.19 \\ \hline
        Average & 16.35 & 18.55 & 7.66 & 4.39 & 5.55 & 9.80 & 0.40 \\ \hline

    \end{tabular}}
\end{table}
